# Supplementary material for: Pattern selection and restricted vortex dynamics by spatial periodic forcing in rapidly rotating Rayleigh-B\'enard convection
Source: arXiv:2201.09492 source file (2022-01-24)
Supplement: Supplementary file 1 [file Supplement.pdf]

# Pattern selection and restricted vortex dynamics by spatial periodic forcing in rotating Rayleigh-Bénard convection

Shan-Shan Ding, Hong-Lin Zhang, Dong-Tian Chen, Hao-Hang Sun, and Jin-Qiang Zhong*
*School of Physics Science and Engineering, Tongji University, Shanghai 200092, China*
(Dated: January 24, 2022)

## I. EXPERIMENTAL APPARATUS AND METHODS

Figure 1a presents a schematic drawing of the experimental apparatus. We used a cylindrical cell mounted on a rotating table. Its bottom plate was made of 35 mm thick oxygen-free copper, heated from below by a uniformly distributed electric wire heater. Seven thermistors were installed inside the bottom plate, one at the center and the other six equally spaced on a circle of 210.0 mm in diameter. The heater was operated in a digital feedback loop in conjunction with these thermistors to hold the bottom-plate temperature constant. Temperature inhomogeneity on the bottom plate was within 1% of the applied temperature difference $\Delta T$ of the cell. The top plate of the cell was a 5 mm thick sapphire disc, cooled from above by a circulating water bath. Four thermistors were installed in the water bath, next to the top side of the sapphire plate. The sidewall of the cell, made of 3 mm thick Plexiglas, was protected against the ambient temperature fluctuations by an adiabatic side shield that maintained a constant temperature of the central fluid. To eliminate the parasitic heat current from the bottom plate to the ambient air, a bottom adiabatic shield was installed under the bottom plate. This thermal shield was covered from below by a heater with a thermistor located at the center of the shield. A second auxiliary heater was wound around the periphery of the bottom shield and its temperature was measured by a second thermistor. Both heaters worked in conjunction with their relevant thermistors to maintain the bottom-shield temperature as the bottom plate. Most of the spatial volume in between the thermal shields and the convection cell was filled with low-density foam to prevent convective air flows. The rotation speed of the table was set in the clockwise direction with the rotational direction pointing downward.

For the present study, we constructed on the bottom plate an array of thin cylinders that extends out from the bottom surface. These raised cylinders were periodically spaced to form a square (Fig. 1b) or hexagon (Fig. 1c) bottom texture. The diameter of these cylinders, $d$=6.0 mm, was approximately equal to the mean diameter of the vortices measured in the reference cell (see Fig. 1a in the main paper). The cylinder height $h$=3.0 mm was chosen close to the thickness of the thermal boundary layer inferred from heat-transport measurement [See Lu et. al., Phys. Rev. Fluids, **6**, L071501 (2021)]. The spacing between adjacent cylinders $\lambda$ was varied as a control parameter of the experiment.

All thermistors installed in the apparatus were calibrated simultaneously in a separate calibration facility with a precision of one or two milli-kelvins against a laboratory standard platinum thermometer traceable to the ITS-90 temperature scale. The onset value of $\Delta T_c$ for convection was determined from the theoretical prediction using an asymptotic method, i.e., $\mathrm{Ra_c}=a\mathrm{Ek}^{-4/3}$, with $a$=8.70−9.63$\mathrm{Ek}^{1/6}$ [P. P. Niiler and F. E. Bisshopp, J. Fluid Mech. **22**, 753 (1965)] ; and also from the measured intensity of the vorticity field in the reference cell (Fig. 3 of the main paper). For $\Omega=1.12\times10^4$, the two determinations of $\Delta T_c$ agreed to within 0.02K.

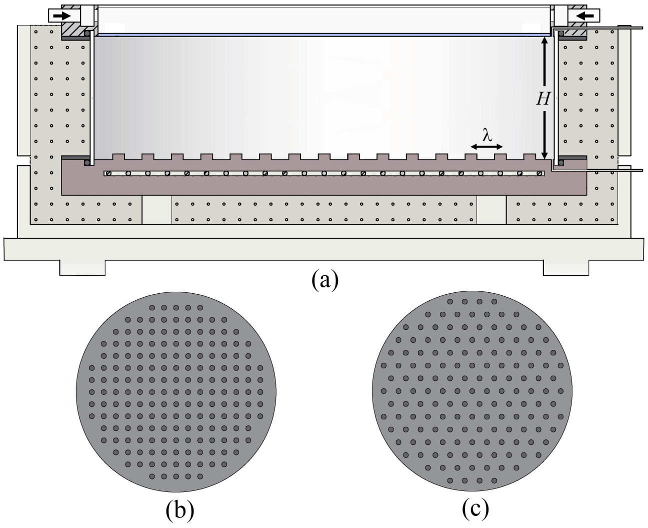


FIG. 1. (a) Schematic of the experimental setup on the rotating table (not to scale). The various components are explained in the text. (b) and (c) Top views of the bottom plate patterned with a square and a hexagonal array of raised cylinders in the forced cells.

For flow visualization, a particle image velocimetry (PIV) system was installed on the co-rotating frame. A thin light-sheet powered by a solid-state laser illuminated the seed particles in a horizontal plane at a fluid height $z=H/4$. Images of the particle were captured through the top sapphire window by a high-resolution

* jinqiang@tongji.edu.cn

camera. Two-dimensional velocity fields were extracted by cross-correlating two consecutive particle images. To increase the accuracy of the vorticity measurements near onset, we chose the measured area as a central region of 65.8×54.8 mm$^2$ over the cross section of the cell, reaching a spatial resolution of 0.64mm in the velocity field. To investigate the long-term stability of the flow pattern near onset (e. g. Figs. 1b and 1c in the main paper), we took image sequences over 8 hours at a time interval of 0.5 second. Our experimental method of PIV has been adopted previously for high-resolution flow structure measurement in rapidly rotating Rayleigh-Bénard convection (RBC) [1–3].

## II. THE AMPLITUDE EQUATIONS

When convection sets in near onset in rotating RBC, various types of patterns form which undergo slow spatiotemporal variation. One feature of these patterns is that they are dominated by finite modes with each mode related to a plane wave (roll) along one certain direction. The strength of these convection modes are constrained by the symmetry of the system, and can be described by a set of nonlinear amplitude equations. One typical flow pattern for rotating RBC near onset is straight convective rolls which is described by a single-mode Ginzburg-Landau equation [4]. Square and hexagonal patterns develop at larger rotating rates $\Omega$, and their spatiotemporal variation are dictated by multiple-mode amplitude equations [5, 6].

In our experiment of rotating RBC with external forcing, we observed regular square and hexagonal flow patterns with prescribed symmetry. As shown in Fig. 2, these convection modes are stationary with the amplitude of each Fourier mode being equal to each other. Based on these observations, we show in the following that the multi-mode amplitude equations describing the observed hexagonal and square patterns can be simplified into one single equation. We first show that the hexagonal pattern can be reconstructed using three plane waves with their characteristic wave vectors $\vec{k}_1$, $\vec{k}_2$, $\vec{k}_3$ equally spaced (see as well Fig. 1f in the main paper). The general variable $q$ of the flow field (e.g., temperature, velocity and vertical vorticity, etc.) can be decomposed into three Fourier modes.

$$q(x,y,z,t)=\sum_{j=1}^{3}A_j(x,y,t)\mathrm{e}^{i2\pi\vec{k}_j\cdot\vec{x}}f(z)+cc. \quad (1)$$

The variable $A_j$ denotes the normalized complex amplitude of a plane wave with a wave vector $\vec{k}_\mathrm{f}$, fulfilling a relationship for the convective heat transport: $|A|^2$=(Nu−1)Ra/Ra$_\mathrm{c}$. Here Nu is the Nusselt number that denotes the dimensionless convective heat flux per unit area. $f(z)$ is an appropriate eigenfunction satisfying the boundary conditions at the top and bottom of the fluid layer.

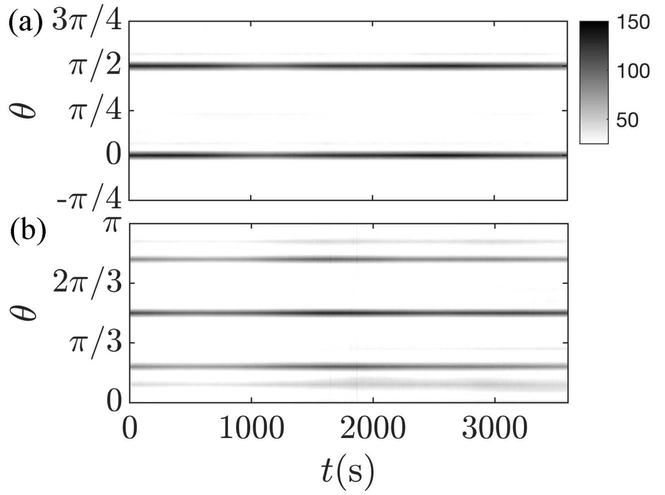


FIG. 2. Angle-time plots for the radial average of the Fourier transformation spectra for (a) the square-patterned cell and (b) the hexagon-patterned cell. Experimental data for $\varepsilon$=0.09 and $\Omega$=1.12 × 10$^4$.

Since the convection flow strength is small near onset, the influence of the imposed bottom texture on the flow field can be understood theoretically by mapping the bottom surface profile to a temperature modulation of the bottom plate [7, 8]. Following the theoretical approach of multiple-mode analysis for flow patterns in rotating RBC [6], we propose a phenomenological Ginzburg-Landau-like model for the convection amplitude $A_j$ in the hexagon-patterned cell:

$$\partial_t A_j=\varepsilon A_j+\xi_0^2\nabla^2 A_j-\sum_{i=1}^{3}g_0^{ij}|A_i|^2A_j+g_2^j\delta_j A_j^{*m-1}. \quad (2)$$

Here $g_0^{ij}$ is the nonlinear coupling coefficient between modes $i$ and $j$. $g_2^j$ is an imperfection coefficient. $\xi_0$ is a spatial gradient coefficient. $g_0^{ij}$ and $g_2^j$ and $\xi_0$ are all dependent on $\vec{k}_\mathrm{f}$ and the applied rotation $\Omega$. $\delta_j$=$c_jh/H$ represents the strength of the external forcing. The coefficient $c_j=\frac{1}{L_xL_y}\int_{-L_x/2}^{L_x/2}\int_{-L_y/2}^{L_y/2}2M(x,y)\cos(2\pi k_j^x x+2\pi k_j^y y)dxdy$ is given by a mask function $M(x,y)$ representing the bottom surface profile (defined in the main text) [7, 8]. We find $c_j^h$=0.172 for the hexagonal texture, and for the square texture $c_j^s$=0.226. $A_j^*$ is the complex conjugate of $A_j$. The integer $m$ denotes the degree of resonance. Since we consider here resonant forcing $k_\mathrm{f}\approx k_0$, $m$=1, and Eq. (2) can be simplified as an amplitude equation:

$$\partial_t A_j=(\varepsilon+\varepsilon_0)A_j-\sum_{i=1}^{3}g_0^{ij}|A_i|^2A_j+g_2^j\delta_j, \quad (3)$$

where $\varepsilon_0$ represents a shift of the convection onset due to

the imposed wave vector $\vec{k}\neq\vec{k}_{\rm f}$ and the slightly increased local temperature gradient over the bottom texture.

We consider stationary solutions $A_j^s$ for Eq. (3). In view of the six-fold symmetry of the hexagonal pattern (see Fig. 1f in the main paper), we have $A_1^s{=}A_2^s{=}A_3^s$. The measured convection amplitude is thus the superposition of the amplitudes of three stationary modes $A{=}\sum_{j=1}^{3} A_j^s$. Denoting the nonlinear coupling coefficient of any two coupling modes $g_0^{ij}$ as a constant $g_0$, the imperfection coefficient $g_2^j$ as $g_2$, and using $\delta^h{=}\sum_{j=1}^{3}\delta_j{=}3\delta_j$, we obtain the amplitude equation of $A$ for the hexagon-patterned cell, through summation of three modes over Eq. (3):

$$(\varepsilon{+}\varepsilon_0^h)A{-}g_0^h|A|^2A/3 + g_2^h\delta^h{=}0. \quad (4)$$

Square flow patterns are unstable as in a bimodal convection state, whereas it is shown that three coupling modes with periodic oscillation resemble stable square patterns in rotating RBC [6]. Nevertheless, our experimental results of the spatiotemporal evolution of the radially averaged Fourier spectra (see Fig. 2a) suggest that the observed square pattern is simply dictated by two stationary modes with their orientations being perpendicular to each other. These results imply that the external forcing is capable to stabilize the bimodal convection state to form square patterns in rotating RBC. In view of the four-fold symmetry of the square pattern (see Fig. 1e in the main paper), we suggest that its measured amplitude, $A{=}\sum_{j=1}^{2} A_j^s$, can be described through summation of two modes over Eq. (3):

$$(\varepsilon{+}\varepsilon_0^s)A{-}g_0^s|A|^2A/2{+}g_2^s\delta^s{=}0, \quad (5)$$

with $\delta^s{=}\sum_{j=1}^{2}\delta_j{=}2\delta_j$. We note that both $g_0^s$ and $g_2^s$ for square pattern differ from those of the hexagonal pattern since they are dependent on $\vec{k}_{\rm f}$.

When the external forcing is absent, $\delta{=}0$ and $\vec{k}_{\rm f}{=}\vec{k}_0$. The amplitude equation for the reference cell is thus reduced to [9]:

$$\varepsilon A{-}g_0^r A^3{=}0, \quad (6)$$

where $g_0^r$ is the nonlinear coupling constant for the reference cell depending on $\vec{k}_0$ and $\Omega$.

According to recent theories of rapidly rotating RBC, the convective vortices, which are the main structures of the flow field, possess similar spatial profiles in their temperature, vertical velocity and vertical vorticity fields [see Portegies et. al. Phys. Fluids **20**, 066602 (2008); Grooms et. al. Phys. Rev. Lett. **104**, 224501 (2010)]. The amplitude $A$ is thus related to the mean vertical vorticity modulus $\langle|\omega|\rangle$ through a scale factor $S$, $A{=}S\langle|\omega|\rangle$, yielding a bifurcation equation for $\langle|\omega|\rangle$ for the hexagon-patterned cell

$$(\varepsilon{+}\varepsilon_0^h)\langle|\omega|\rangle{-}g_0^hS^2\langle|\omega|\rangle^3/3{+}g_2^h\delta^hS^{-1}{=}0, \quad (7)$$

for the square-patterned cell

$$(\varepsilon{+}\varepsilon_0^s)\langle|\omega|\rangle{-}g_0^sS^2\langle|\omega|\rangle^3/2{+}g_2^s\delta^sS^{-1}{=}0, \quad (8)$$

| | $\varepsilon_0$ | $g_0S^2[s^2]$ | $g_2\delta S^{-1}$ or $c_0$ $[s^{-1}]$ |
|---|---|---|---|
| Hex. Cell | $1.26{\times}10^{-2}$ | $6.81{\times}10^2$ | $5.00{\times}10^{-4}$ |
| Squ. Cell | $1.00{\times}10^{-3}$ | $4.16{\times}10^2$ | $4.38{\times}10^{-4}$ |
| Ref. Cell | | $2.60{\times}10^2$ | $7.89{\times}10^{-5}$ |

TABLE I. Experimental results of the parameters in the amplitude equations (7), (8) and (9) for the hexagon-patterned (Hex.) cell with $\lambda$=17.32 mm, the square-patterned (Squ.) cell with $\lambda$=14.14 mm and the reference (Ref.) cell.

and for the reference cell

$$\varepsilon\langle|\omega|\rangle{-}g_0^rS^2\langle|\omega|\rangle^3{=}0. \quad (9)$$

Since the intensity of the vorticity field is fluid-depth dependent [Grooms et. al. Phys. Rev. Lett. **104**, 224501 (2010)], the scale factor $S$ depends on the measured fluid height. In measuring $\langle|\omega|\rangle$ we choose strictly a measurement height at $z{=}H/4$ for both the reference cell and the forced cells, utilizing the same PIV settings in the experiment. Therefore, $S$ remains a constant parameter for all measurements.

We fitted the experimental data of $\langle|\omega|\rangle(\varepsilon)$ to the theoretical predictions of Eqs. (7-9) for the forced cells and the reference cell, respectively (see Fig. 3 in the main paper). Results of the fitting parameters are summarized in Table 1. In the following we make discussions of these parameters and compare them with theoretical predictions wherever possible.

**Coefficients $g_0, g_2$ and the scale factor $S$**

Fitting the experimental data $\langle|\omega|\rangle(\varepsilon)$ of the reference cell, we determine the coefficient of the cubic term in Eq. (9), $g_0^rS^2{=}2.60{\times}10^2[s^2]$. The scale factor $S$ is thus related to $g_0^r$ through: $S{=}16.12[s]/\sqrt{g_0^r}$. According to Eqs. (7) and (8), we find also for the square-patterned and hexagon-patterned cells $g_0^sS^2{=}4.16{\times}10^2[s^2]$ and $g_0^hS^2{=}6.81{\times}10^2[s^2]$, respectively. They thus lead to the following relationship: $g_0^s{=}4.16{\times}10^2[s^2]S^{-2}$ and $g_0^h{=}6.81{\times}10^2[s^2]S^{-2}$. Using Eqs. (7) and (8) one obtains as well the constant term representing the effect of imperfect bifurcation, $g_2^s\delta^sS^{-1}{=}4.38{\times}10^{-4}[s^{-1}]$ for the square-patterned cell, and $g_2^h\delta^hS^{-1}{=}5.00{\times}10^{-4}[s^{-1}]$ for the hexagon-patterned cell. Given by the values of $\delta^s{=}0.0215$ and $\delta^h{=}0.0246$, we find $g_2^s{=}2.04{\times}10^{-2}[s^{-1}]S$ and $g_2^h{=}2.03{\times}10^{-2}[s^{-1}]S$.

We define a bifurcation parameter, $G{=}\sqrt{g_0}g_2$, which reveals the transitional property of the bifurcation curve $\langle|\omega|\rangle(\varepsilon)$ near onset. We find for the two forced cells $G_s{=}\sqrt{g_0^s}g_2^s{=}0.416$, $G_h{=}\sqrt{g_0^h}g_2^h{=}0.530$, both are independent of the scale factor $S$.

To our knowledge, there exists yet no complete theory of near-onset bifurcation for rotating convection with periodic external forcing. Kelly and Pal derived the amplitude equation of non-rotating RBC subjected to a spatially sinusoidal modulation [7]. They showed that the external modulation results in an imperfection

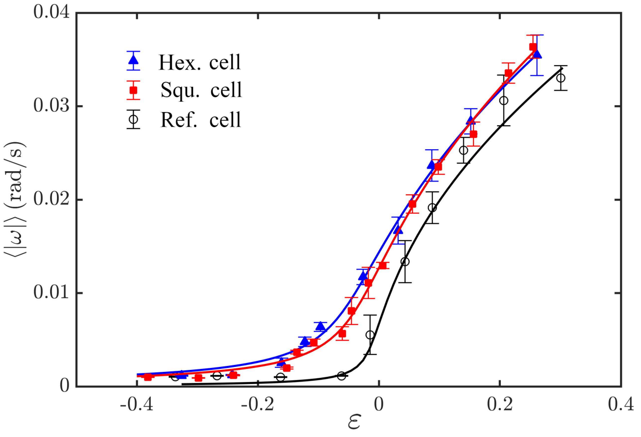


FIG. 3. Bifurcation curves of $\langle|\omega|\rangle(\varepsilon)$ for the reference cell (black circles), the square-patterned cell (red squares) with $\lambda$=14.14 mm, and the hexagon-patterned cell (blue triangles) with $\lambda$=17.32 mm. Results for $\Omega$=1.12×10$^4$. The solid curves are the fitted imperfect bifurcation curves predicted by Eq. (7) and (8) for the forced cells and Eq. (9) for the reference cell. Error bars denote the standard deviation.

term in the amplitude equation, and determined the imperfection coefficient $g_2^{RB}$=0.144, and the cubic term coefficient, $g_0^{RB}$=13.05 in their units (see also [10]). Therefore, the theoretically predicted value of the bifurcation parameter for non-rotating RBC, $G_{RB}=\sqrt{g_2^{RB}g_0^{RB}}=0.520$, appears close to our results of $G_s$ and $G_h$ for the square- and hexagon-patterned cells in rotating convection.

### Offset of the convection onset $\varepsilon_0$

In the reference cell the flow exhibits a convection pattern with an intrinsic wave number $k_0$ near onset, and the onset of convection is given by $\mathrm{Ra_c}=a\mathrm{Ek}^{-4/3}$, with $a$=8.70−9.63Ek$^{1/6}$. When periodic external forcing is present, however, the convection pattern is dictated by the imposed wave vector $\vec{k}_\mathrm{f}$. A small shift of the onset $\varepsilon_0$ may occur if $k_\mathrm{f}\neq k_0$ [9]. Furthermore, the imposed bottom texture in the present study increase slightly the local temperature gradient that may also influence $\mathrm{Ra}_c$ [8, 10]. Fitting our experimental data of $\langle|\omega|\rangle(\varepsilon)$ to Eqs. (7) and (8) we find the onset of convection is offset by $\varepsilon_0^s$=1.0×10$^{-3}$ and $\varepsilon_0^h$=1.26×10$^{-2}$ for the square- and hexagon-patterned cells, respectively. Since $\varepsilon_0^s$ and $\varepsilon_0^h$ are two or three orders in magnitude less than unity, we conclude that the external forcing has a negligible effect on the onset of convection.

### The imperfection parameters

Owing to the influence of static sidewall forcing in realistic experiments, a slight rounding of the bifurcation in the reference cell may occurs. We use a parameter $c_0$ to model this sidewall effect [10]:

$$\varepsilon\langle|\omega|\rangle - g_0^r S^2\langle|\omega|\rangle^3 + c_0 = 0. \quad (10)$$

In Fig. 3, we fit experimental data of $\langle|\omega|\rangle(\varepsilon)$ from the reference cell to Eq. (10), and determine the parameter $c_0$. We obtain $c_0$=7.89×10$^{-5}$, which is one order of magnitude smaller than the imperfect parameter $g_2\delta/S$ of the two forced cells. This result implies that the sidewall effect is minor and the transition near onset of the reference cell is relatively sharp, in contrast with the pronounced rounding of the transition in the forced cells. The fluid flows induced by wall-mode convection, or by the boundary zonal flows [11–13], may have influence on the vorticity field in the central region of convection cells with finite $\Gamma$ [see e. g., Marques et. al. Phys. Fluids, **20**, 024109, 2008], leading to a non-zero imperfection parameter $c_0$. We expect that a strictly perfect bifurcation near the onset of rotating convection can be observed only in infinitely extended (laterally unbounded) systems.

### The background signal of the vorticity field

Due to the finite resolution of our PIV system, a finite background signal of the vorticity field $\langle|\omega|\rangle(0)$ exists even when the applied temperature difference is zero. With $\Delta T$=0.00$K$ we determine the magnitude of this background signal, $\langle|\omega|\rangle_{\Delta T=0}\approx$1.0×10$^{-3}$ rad/s, which is at the same level of $\langle|\omega|\rangle(\varepsilon)$ in the reference cell when $\varepsilon<0$, but one order in magnitude less than $\langle|\omega|\rangle(\varepsilon)$ in the forced cells for $\varepsilon\approx0$. Therefore, the background signal does not alter the above conclusions of our bifurcation analysis.

## III. CALCULATIONS OF THE VORTEX DIFFUSION COEFFICIENT

The dynamics of the vortices in the forced cells undergoes a transition from Brownian motion with strong thermal forcing ($\varepsilon\geq$5.0), to anomalous diffusive motion when thermal forcing is weakened near onset. In the anomalous diffusion regime, the mean-square displacements of the cyclonic vortices vary in large time scale as $\delta\vec{r}^2(t)=t^\gamma$, with the exponent $\gamma<1$. Apparently this subdiffusive behavior of cyclones is ascribed to the modulation effects from the external forcing, i.e., cyclones are confined above the raised cylinders, while anticyclones are restricted from moving above the cylinders (see Fig. 4 in the main paper). In Figs. 4a and 4b we show for various $\varepsilon$, the velocity auto-correlation function of cyclones and anticyclones, respectively, $V(t)=\langle\vec{u}(0)\cdot\vec{u}(t)\rangle$. We find that in a very short time scale, $V(t)$ decreases approximately as an exponential function of time, $V(t)=V_0e^{-t/t_c}$ [2]. After two or three characteristic time scale of ballistic motion ($t\leq2\sim3t_c$), $V(t)$ becomes a non-monotonic function of time, and exhibits oscillatory behavior for some cases at large time. The apparent non-monotonic behavior of $V(t)$ reveals the modulated vortex motion under external forcing.

To quantify in general the movability of the vortices under various strength of external forcing, we calculate

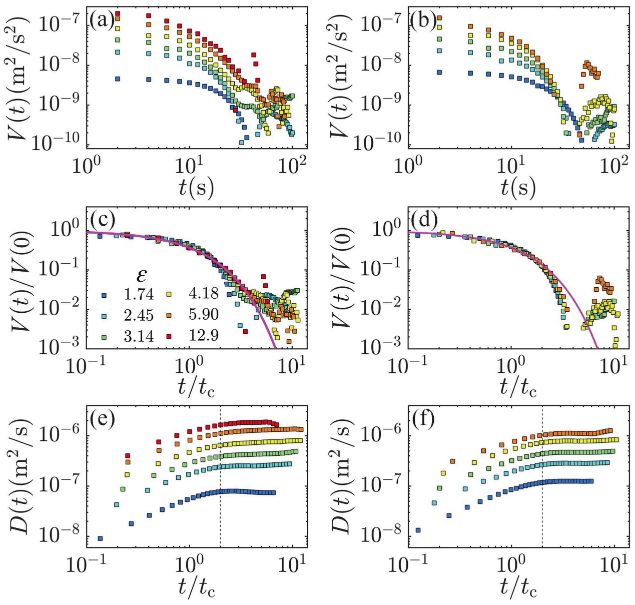


FIG. 4. (a, b) The velocity auto-correlation functions $V(t)$ of vortex motion as a function for time for various $\varepsilon$. (c, d) The scaled velocity auto-correlation functions $V(t)/V(0)$ as a function for $t/t_c$. The solid line represents an exponential fit to the data, $V(t)=V(0)e^{-t/t_c}$. (e, f) The diffusivity of vortex motion as a function of $t/t_c$. The dashed line indicates $t=2t_c$. Results are for the square-patterned cell with $\lambda=14.14$ mm and $\Omega=1.12\times10^4$. (a,c,e) are data for the cyclones and (b,d,f) for the anticyclones. Legends are shown in (c).

the time-dependent diffusivity $D(t)$ of the vortices, which is related to $V(t)$ through the Green-Kubo formula, $D(t)=\int_0^t V(t')dt'$. Figures 4e and 4f present results of $D(t)$ for cyclones and anticyclones, respectively. We see that for various thermal forcing $D(t)$ first increases with time in a short time scale, then approaches a constant after $t>t_c$. The rapid convergence of the value of $D(t)$ is associated with the non-monotonic, oscillating values of $V(t)$ around zero at large time. Finally, we determine the asymptotic diffusion coefficient of vortex motion, $D=\lim_{t\to\infty} D(t)$, taking the time-average of $D(t)$ with $t\geq 2t_c$. Results of $D$ are shown as a function of $\varepsilon$ in the Fig. 4 insets of the main paper. The uncertainty in determining $D$ is estimated using the standard deviation of $D(t)$ for $t\geq 2t_c$.

## IV. SUPPLEMENTARY MOVIES

Movie 1. Experimental movie corresponding to Fig. 1a in the main paper. The movie shows the distributions of vorticity fields over a horizontal cross-section of the reference cell at $z=H/4$. Results for $\Omega=1.12\times10^4$ and $\varepsilon=0.49$.

Movie 2. Experimental movie corresponding to Fig. 1b in the main paper. Results of $\omega(t)$ over a horizontal cross-section of the square-patterned cell at $z=H/4$ for $\Omega=1.12\times10^4$ and $\varepsilon=0.49$.

Movie 3. Experimental movie corresponding to Fig. 1c in the main paper. Results of $\omega(t)$ over a horizontal cross-section of the hexagon-patterned cell at $z=H/4$ for $\Omega=1.12\times10^4$ and $\varepsilon=0.49$.


[1] J.-Q. Shi, H.-Y. Lu, S.-S. Ding, and J.-Q. Zhong, Phys. Rev. Fluids **5**, 011501(R) (2020).

[2] K. L. Chong, J.-Q. Shi, S.-S. Ding, G.-Y. Ding, H.-Y. Lu, J.-Q. Zhong, and K.-Q. Xia, Sci. Adv. **6**, eaaz1110 (2020).

[3] S.-S. Ding, K. L. Chong, J.-Q. Shi, G.-Y. Ding, H.-Y. Lu, K.-Q. Xia, and J.-Q. Zhong, Nat. Commun. **12**, 5585 (2021).

[4] J. D. Scheel, Phys. Fluids **19**, 104105 (2007).

[5] H. F. Goldstein, E. Knobloch, and M. Silber, Phys. Rev. A **48**, 4755 (1992).

[6] J. D. Scheel, P. L. Mutyaba, and T. Kimmel, J. Fluid Mech. **659**, 24 (2010).

[7] R. E. Kelly and D. Pal, J. Fluid Mech. **86**, 433 (1978).

[8] G. Seiden, S. Weiss, J. H. McCoy, W. Pesch, and E. Bodenschatz, Phys. Rev. Letts. **101**, 214503 (2008).

[9] M. C. Cross, Phys. Fluids **23**, 1727 (1980).

[10] J. H. McCoy, *Pattern Forming System in the Presence of Different Symmetry-Breaking Mechanisms*, Ph.D. thesis, Cornell University (2007).

[11] F. Zhong, R. Ecke, and V. Steinberg, Phys. Rev. Letts. **67**, 2473 (1991).

[12] X. M. de Wit, A. J. Aguirre Guzmán, M. Madonia, J. S. Cheng, H. J. H. Clercx, and R. P. J. Kunnen, Phys. Rev. Fluids **5**, 023502 (2020).

[13] X. Zhang, D. P. M. van Gils, S. Horn, M. Wedi, L. Zwirner, G. Ahlers, R. E. Ecke, S. Weiss, E. Bodenschatz, and O. Shishkina, Phys. Rev. Lett. **124**, 084505 (2020).
